# Supplementary material for: Learning to Stabilize Unknown LTI Systems on a Single Trajectory under Stochastic Noise
Source: arXiv:2406.00234 source file (2024-05-31)
Supplement: Supplementary file 1 [file Appendix_ls_lemmas.tex]

\begin{lemma}
    \begin{equation*}
        (P_1' DD' P_1)(D D')^{-1} = I + 
    \end{equation*}
\end{lemma}
\begin{proof}
We first expand out $P_1' DD' P_1$. Since $D = Q \begin{bmatrix}
    D_1 \\ D_2
\end{bmatrix}$, we get
    \begin{align*}
        P_1' DD' P_1 =& P_1'\begin{bmatrix}
            Q_1 & Q_2 
        \end{bmatrix}
        \begin{bmatrix}
            D_1 \\ D_2
        \end{bmatrix}
        \begin{bmatrix}
            D_1' & D_2'
        \end{bmatrix}
        \begin{bmatrix}
            Q_1' \\ Q_2'
        \end{bmatrix}
        P_1
        \\
         =& \begin{bmatrix}
            I & P_1' Q_2
        \end{bmatrix}
        \begin{bmatrix}
            D_1 D_1' & D_1 D_2' \\ D_2 D_1' & D_2 D_2'
        \end{bmatrix}
        \begin{bmatrix}
            I \\ Q_2' P_1
        \end{bmatrix}
        \\
         =& D_1 D_1' + P_1' Q_2 D_2 D_1' + D_1 D_2' Q_2' P_1 
        \\
        &+ P_1'Q_2 D_2 D_2' Q_2' P_1
    \end{align*} 
    We then bound the last three terms above separately.
    \begin{align*}
        \norm{P_1' Q_2 D_2 D_1'} &\leq \norm{P_1' Q_2 D_2} \norm{D_1'} \\
        &\leq T(n-k) \frac{C}{1 - |\lambda_{k+1}|} k \sum_{t=1}^T |\lambda_1^k C|
    \end{align*}
\end{proof}

\begin{lemma}
    If $\eta \in \mathbb{R}^k$ is a sub-Gaussian vector with parameter $r$, $G \eta$ is sub-Gaussian with parameter $r$.
\end{lemma}
\begin{proof}
    By definition, for any $x \in \mathbb{R}^k$, 
    \begin{equation*}
        \E\left[e^{x' \eta}|\mathcal{F}_{t-1}\right] \leq \exp\left(\frac{\norm{x}^2 r^2}{2}\right).
    \end{equation*}
    Therefore,
    \begin{align*}
        \E\left[e^{x' (G\eta)}\right] &= \E\left[e^{(G' x)' \eta_t}\right] 
        \\
        & \leq \exp\left(\frac{\norm{x}^2 (\sigma_1(G) r)^2}{2}\right)
    \end{align*}
\end{proof}
